# Supplementary material for: Learning compositional structures for semantic graph parsing
Source: arXiv:2106.04398 source file (2021-06-08)
Supplement: Supplementary file 2 [file appendix-percolations-old.tex]

\section{Details on percolations and unrolling}\label{app:percolations}
\subsection{Percolations}

Fig.~\ref{fig:percolations} shows the three types of percolations \textbf{P1-4} that are applicable in an AM dep-tree. With that we mean, these are all operations that move a node up in a tree or remove a reference node, without changing the 

\textbf{P1} and \textbf{P2} are the two percolation steps we saw in the example in Fig.~6 of the main document. Both apply to a tree node (corresponding to a graph node \nn{n}) with an incoming \app{} edge, whose parent (corresponding to a graph node \nn{p}) also has an incoming \app{} edge from a node (the grandparent of the original tree node) corresponding to a graph node \nn{g}. Both percolations add \ps{n} to the \ps{p}-request at the grandparent, indicating that the parent will have an unfilled \ps{n} source at the time of application.

This is where the commonalities end. \textbf{P1} applies in the case where the grandparent does \emph{not} have a \ps{n} source in its type yet; \textbf{P2} when it \emph{does}.\textbf{P1} applies to any node (original constant or referent for \nn{n}) and attaches its incoming edge at the grandparent instead of the parent.\textbf{P2} applies only to reference nodes and deletes them. This is because the\ps{n} source of the grandparent is already getting filled by an \nn{n}-alias, and the additional reference node is no longer required.

\textbf{P3} is like \textbf{P2} but percolates past a \modify{} edge. Due to how \modify{} operations create reentrancies (c.f. \newcite{groschwitz-etal-2017-constrained}), no type changes occur in \textbf{P3}.

\textbf{P4} is like \textbf{P1} but within a modifier component. It only \sortof{switches} two nodes and cannot be used to resolve reentrancies.

These are all percolations that exist. To see this, we make a case distinction on the bottom edge in the schema, the top edge, and whether the grandparent has \ps{n} in its type.

\begin{description}
\item[Case 1] If the bottom edge is \app{}:
    \begin{description}
    \item[Case 1a] If the top edge is \app{}:
    
        \begin{description}
            \item[Case 1a+] If the grandparent has \ps{n} in its type: \textbf{P2} applies;
            \item[Case 1a-] If the grandparent does not have \ps{n} in its type: \textbf{P1} applies;
        \end{description}

    \item[Case 1b] If the top edge is \modify{}:
        \begin{description}
            
            \item[Case 1b+] If the grandparent has \ps{n} in its type: \textbf{P3} applies
            \item[Case 1b-] If the grandparent does not have \ps{n} in its type: percolation not possible, since \modify{} cannot add a source to the head's type \citep{groschwitz-etal-2017-constrained};
        \end{description}
    \end{description}

\item[Case 2] If the bottom edge is \modify{}:

    \begin{description}
        \item[Case 2a] If the top edge is \app{}: percolation not possible, since it would change which head the node modifes; i.e.~change the evaluation result;
        \item[Case 2b] If the top edge is \modify{}:
        \begin{description}
            \item[Case 2b+] If the grandparent has \ps{n} in its type: this can never happen since the original (edge-normalized) graph would have been cyclic;
            \item[Case 2b-] If the grandparent does not have \ps{n} in its type: \textbf{P4} applies.
        \end{description}
    \end{description}
\end{description}


\subsection{Algorithm for unrolling a graph}
We use the following algorithm to obtain exactly the unrolled graphs that lead to valid AM dep-trees.

% graph unrolling
\begin{figure}
    \centering
    \begin{subfigure}[b]{0.3\linewidth}
        \includegraphics[scale=\bigAMRScale]{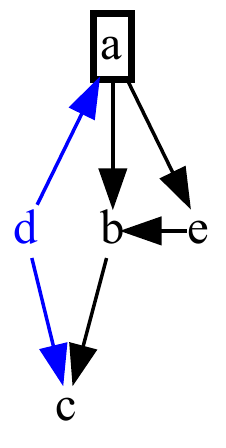}
        \caption{}
    \end{subfigure}
    \begin{subfigure}[b]{0.3\linewidth}
        \includegraphics[scale=\bigAMRScale]{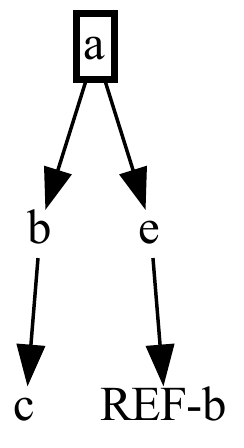}
        \caption{}
    \end{subfigure}
    \begin{subfigure}[b]{0.33\linewidth}
        \includegraphics[scale=\bigAMRScale]{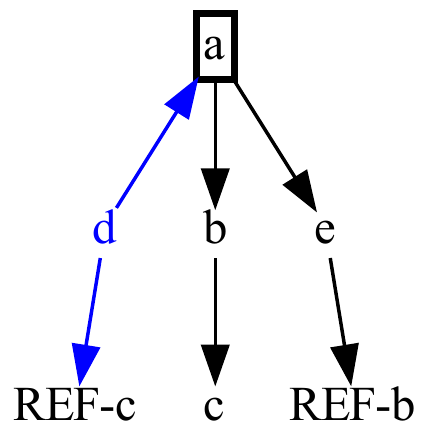}
        \caption{}
    \end{subfigure}
    \caption{(a) Graph $G$, (b) after forward expansion and (c) fully unrolled. We leave out node and edge labels here for readability.}
    \label{fig:unroll}
\end{figure}

% Trees
\begin{figure}
    \centering
    %P1.1
    \begin{subfigure}[b]{0.45\linewidth}
    \centering
        \begin{forest}
        for tree={align=center, edge=->, l sep=2em, l=2em, }
        [\depNodeWType{\nn{g}}{\type{\ps{p}}}
            [\depNodeWType{\nn{p}}{\type{\ps{n}}}, edge label = {node [midway, left] {\app{\ps{p}}}}
                [\depNodeWType{\nn{n}}{\emptytype}, edge label = {node [midway, left] {\app{\ps{n}}}}
                ]
            ]
        ]
        \end{forest}
    \caption{\textbf{P1} before}
    \end{subfigure}
    % P1.2
    \begin{subfigure}[b]{0.5\linewidth}
    \centering
        \begin{forest}
        for tree={align=center, edge=->, l sep=2em, l=2em, }
        [\depNodeWType{\nn{g}}{\type{\ps{p}\type{\ps{n}}}}
            [\depNodeWType{\nn{n}}{\emptytype}, edge label = {node [midway, left] {\app{\ps{n}}}}
            ]
            [\depNodeWType{\nn{p}}{\type{\ps{n}}}, edge label = {node [midway, right] {\app{\ps{p}}}}
            ]
        ]
        \end{forest}
    \caption{\textbf{P1} after}
    \end{subfigure}
    % P2.1
    \begin{subfigure}[b]{0.45\linewidth}
    \centering
        \begin{forest}
        for tree={align=center, edge=->, l sep=2em, l=2em, }
        [\depNodeWType{\nn{g}}{\type{\ps{p,n}}}
            [\depNodeWType{\nn{p}}{\type{\ps{n}}}, edge label = {node [midway, left] {\app{\ps{p}}}}
                [\depNodeWType{\refnode{n}}{\emptytype}, edge label = {node [midway, left] {\app{\ps{n}}}}
                ]
            ]
        ]
        \end{forest}
    \caption{\textbf{P2} before}
    \end{subfigure}
    %P2.2
    \begin{subfigure}[b]{0.5\linewidth}
    \centering
        \begin{forest}
        for tree={align=center, edge=->, l sep=2em, l=2em, }
        [\depNodeWType{\nn{g}}{\type{\ps{p\type{\ps{n}},n}}}
            [\depNodeWType{\nn{p}}{\type{\ps{n}}}, edge label = {node [midway, left] {\app{\ps{p}}}}
            ]
        ]
        \end{forest}
    \caption{\textbf{P2} after}
    \end{subfigure}
    %P3.1
    \begin{subfigure}[b]{0.45\linewidth}
    \centering
        \begin{forest}
        for tree={align=center, edge=->, l sep=2em, l=2em, }
        [\depNodeWType{\nn{g}}{\type{\ps{n}}}
            [\depNodeWType{\nn{p}}{\type{\ps{n,g}}}, edge label = {node [midway, left] {\modify{\ps{g}}}}
                [\depNodeWType{\refnode{n}}{\emptytype}, edge label = {node [midway, left] {\app{\ps{n}}}}
                ]
            ]
        ]
        \end{forest}
    \caption{\textbf{P3} before}
    \end{subfigure}
    %P3.2
    \begin{subfigure}[b]{0.5\linewidth}
    \centering
        \begin{forest}
        for tree={align=center, edge=->, l sep=2em, l=2em, }
        [\depNodeWType{\nn{g}}{\type{\ps{n}}}
            [\depNodeWType{\nn{p}}{\type{\ps{n,g}}}, edge label = {node [midway, left] {\modify{\ps{g}}}}
            ]
        ]
        \end{forest}
    \caption{\textbf{P3} after}
    \end{subfigure}
    %P4.1
    \begin{subfigure}[b]{0.45\linewidth}
    \centering
        \begin{forest}
        for tree={align=center, edge=->, l sep=2em, l=2em, }
        [\depNodeWType{\nn{g}}{\emptytype}
            [\depNodeWType{\nn{p}}{\type{\ps{g}}}, edge label = {node [midway, left] {\modify{\ps{g}}}}
                [\depNodeWType{\nn{n}}{\type{\ps{p}}}, edge label = {node [midway, left] {\modify{\ps{p}}}}
                ]
            ]
        ]
        \end{forest}
    \caption{\textbf{P4} before}
    \end{subfigure}
    \begin{subfigure}[b]{0.5\linewidth}
    \centering
        \begin{forest}
        for tree={align=center, edge=->, l sep=2em, l=2em, }
        [\depNodeWType{\nn{g}}{\emptytype}
            [\depNodeWType{\nn{n}}{\type{\ps{p}\type{\ps{g}}}}, edge label = {node [midway, left] {\modify{\ps{g}}}}
                [\depNodeWType{\nn{p}}{\type{\ps{g}}}, edge label = {node [midway, left] {\app{\ps{p}}}}
                ]
            ]
        ]
        \end{forest}
    \caption{\textbf{P4} after}
    \end{subfigure}
    \caption{Schematic representations of the percolations \textbf{P1-4}. Nodes in the AM dep-trees do not show the constant, but a pair \nn{n}: $\tau$ of the graph node corresponding to the constant, and the constant's type (in practice the type may contain additional sources).}
    \label{fig:percolations}
\end{figure}



Consider the graph $G$ in Fig~\ref{fig:unroll}a as an example. We start at the root $a$ of $G$ and perform a \emph{forward expansion}, where we traverse edges in forward direction and breadth first order as far as possible. We add nodes and edges to the unrolled graph $U$ as we pass them. When we see a node for the second time, we add a reference node to $U$ instead (and don't traverse the node's outgoing edges again); see Fig~\ref{fig:unroll}b for the result. The exact order of this expansion does not matter, since a node and all its reference will get percolated up to the same lowest common ancestor in any case.

This forward expansion may leave us with several connected components $C_i$ of nodes that have not been traversed; here, we have one such component $C_0$ containing exactly the node \nn{d}. Each edge connecting a $C_i$ to the rest of the graph has its origin in $C_i$ (if the edge went the other way, it would have been traversed during the forward expansion). We write $D_i$ for the set of nodes not in $C_i$ with an incoming edge from $C_i$; in this example, $D_0=\left\{\nn{a},\nn{c}\right\}$. We then traverse one edge from the \emph{lowest common ancestor} of $D_i$ into $C_i$ -- this traverses the edge in backwards direction -- arriving at a node $r_i$. We then continue the forward expansion process starting at $r_i$, continuing this iteration until all nodes are covered. In the example, the lowest common ancestor of $D_0$ is \nn{a}, and we accordingly traverse from \nn{a} to $r_0=\nn{d}$, traversing backwards across the edge. We then continue the forward expansion from there, adding a reference node to \nn{c} and obtaining the final unrolled graph in Fig~\ref{fig:unroll}c.

Note that the backwards traversed edge between \nn{a} and \nn{d} turns into a \modify{} edge in the canonical AM dep-tree, since it points towards the root. Further recall that we can percolate \refnode{\nn{c}} past that edge only if the constant \constof{\nn{a}} its parent \nn{a} has an \ps{\nn{c}} source. This is not the case naturally -- \constof{\nn{a}} has arguments \nn{b} and \nn{e} -- but we can get the source \ps{\nn{c}} in there by percolating \nn{c} upwards past \nn{b}. This is possible because \nn{a} is an ancestor of \nn{b}, which is why we choose the lowest common ancestor of $D_i$ as the node from which to traverse into $C_i$. If there are multiple edges from $C_i$ to that lowest common ancestor, we can choose any one, each yielding a different AM dep-tree in the end. If there is no such edge, there is no AM dep-tree for this choice of blob partition and the decomposition fails.
